# Supplementary material for: On Difficulties of Cross-Lingual Transfer with Order Differences: A Case Study on Dependency Parsing
Source: arXiv:1811.00570 source file (2019-04-17)
Supplement: Supplementary file 1 [file main-appendix.tex]

% separately build for appendix

\documentclass[11pt,a4paper]{article}
\usepackage[hyperref]{naacl2019}
\usepackage{times}
\usepackage{latexsym}

\usepackage{longtable}
\usepackage{makecell}

\usepackage{hyperref}
\usepackage{url}
\usepackage{comment}
\usepackage[flushleft]{threeparttable}
\usepackage{graphicx}
\usepackage{amsmath}
\usepackage{subfig}
\usepackage{tabularx}
\usepackage{multirow}
\usepackage{algorithm}
\usepackage{enumitem}
\usepackage{todonotes}

\linespread{1.0}

\aclfinalcopy

\begin{document}

\cleardoublepage
\input{appendix}

\bibliography{naacl2019}
\bibliographystyle{acl_natbib}

\end{document}
